# Supplementary material for: Realistic Full-Body Anonymization with Surface-Guided GANs
Source: arXiv:2201.02193 source file (2023-06-01)
Supplement: Supplementary file 1 [file coco_additional_details.tex]

\section{COCO Anonymization Details}
\label{sec:coco_appendix}
The anonymization framework consists of two stages, detection and generation.

The detection network is a pre-trained CSE \cite{neverova2020cse} network \footnote{Specifically, \href{https://github.com/facebookresearch/detectron2/blob/main/projects/DensePose/configs/cse/densepose_rcnn_R_101_FPN_DL_s1x.yaml}{R-101-FPN-DL-s1x}.} from detectron2 \cite{wu2019detectron2}.
We detect pixel-to-surface correspondences on the entire image (can contain several identities), then crop every person out.
For each instance detected, we crop by first finding the minimum bounding box that contains the detected surface, then expand this surface to a rectangular shape that has a similar aspect ratio of the target resolution ($288 \times 160)$.
In addition, we ensure that 30\% of the resulting crop contains "background" (\ie not the surface).
We zero-pad the image if there is no possible crop that fits in the original image.

We crop the CSE-embedding similarly.
The cropped image and the embedding is then resampled to $288 \times 160$ with bilinear up/downsampling.
The segmentation map $S$ outputted by CSE is 1 for every pixel belonging to the surface.
We equally resample $S$ and dilate $S$ depending on the number of pixels in the image that belongs to the surface.
This is to ensure that we remove clothing and other accessories on the human body, as CSE primarily detects the body.
Then, we zero-out all pixels that are belongs to the surface, indicated by the dilated segmentation $S$.
The resulting partial image is the input of our surface-guided generator.

The final image is naively stitched together.
For each instance, the generated image is resampled to the original resolution, then all pixels in the original image belonging to the dilated surface is replaced by with the generated ones.

\subsection{COCO-Body Dataset}
We generate the COCO-Body dataset by using the detection procedure described above on COCO \cite{lin2014microsoft} train2014 and val2014.
Specifically, for every image in the COCO dataset, we detect instances in the image.
For each instance, we find the cropped image (described above) and include the image in the dataset if either; (1) the detected surface has more than 80\% geodisic point similarity \cite{Guler_2018} to the ground truth DensePose-CSE dataset \cite{neverova2020cse}, or (2) the instance has a confidence score higher than $99.5\%$.
Out of these detections, we filter out all images that are not in the aspect ratio range $[0.4, 4]$ (height/width), images that cover an area smaller than $144 \times 80\;$ pixels, or images that contains more than $25\%$ zero-padding (in image area).

After filtering the detections, we are left with $43,053\;$ images from COCO train2014, and $10,777$ in val2014.
We use this train/validation split for our experiments.
The dataset is published open source at \href{https://github.com/hukkelas/full_body_anonymization}{github.com/hukkelas/full\_body\_anonymization}.
