# Supplementary material for: Realistic Full-Body Anonymization with Surface-Guided GANs
Source: arXiv:2201.02193 source file (2023-06-01)
Supplement: Supplementary file 2 [file experimental_details.tex]

\section{Additional Experimental Details}
\label{sec:app_experimental_details}
We describe the general setup of  the COCO-Body model here and state specific changes to DeepFashion in Sec. A.3.

All experiments were performed with Pytorch v1.11 \cite{paszke2019pytorch} with 2x Tesla V100-32GB GPUs.
FID and PPL is computed with torch fidelity \cite{torchfidelity}, where we modify the code to support conditional image synthesis.

\subsection{Network Architecture and Hyperparameters}
We use equalized learning rate \cite{karras2018progressive} for all trainable parameters and use the Adam \cite{adam} optimizer with batch size=32, learning rate=0.001, $\beta_1=0.0, \beta_2=0.99$ and $\epsilon=10^{-8}$.
Note that we set the learning rate to 0.002 for Config E.
Each model is trained until the discriminator has seen 12M images.
All networks are trained  with mixed precision using the implementation provided by Pytorch  \cite{paszke2019pytorch}.

\paragraph{Generator Architecture}
The generator architecture is a U-Net architecture \cite{ronneberger2015u} following design principles of StyleGAN2 \cite{karras2019analyzing}.
There are 5 residual blocks in the encoder and 5 in the decoder, where each block has two 3x3 convolutions.
The residual blocks has the following number of output channels (Config E): $[128, 256, 512, 512, 512,512, 512, 256, 128, 64]$.
Convolutions  of the same block has the same number of output channels.
For other configs, we straightforward scale down the reported output channels to match the number of parameters reported in the main paper.
Bilinear upsampling/downsampling is performed after each block (except the end/start of the encoder/decoder).
We use $1 \times 1$ residual skip connections between the first 4 and last 4 blocks of the encoder/decoder.
Each convolution in the residual blocks (except reisdual/u-net skip connections) has the following order of operations; SAM feature modulation $\rightarrow$ convolution $\rightarrow$ LeakyReLU (slope=.2) \cite{leakyReLU} $\rightarrow$ normalization.

The input image resolution is $288 \times 160$ and the minimum feature map resolution is $36 \times 20$.
For inference, we use the exponential moving average \cite{yazici2018the} of the generator, where we use $\beta =0.9977$.
For all models (except those with \modulationMetodNoiseShort, INADE \cite{tan2021INADE}, Co-mod \cite{zhao2021comodGAN} or StyleGAN \cite{karras2019analyzing}), we linearly project the latent variable to a $1 \times 32 \times 32$, then add it to the output of the encoder.

\paragraph{FPN-Discriminator}
The FPN-discriminator consists of 6 residual blocks, with the following number of output channels (Config E) for each: $[128, 256, 512, 512, 512, 512]$, which results in 34M parameters.
For the FPN-Head, we add a $1 \times 1$ convolution that linearly transforms the output of each residual block to the number of output channels (16 for CSE embedding, 26 for semantic segmentation).
These feature maps are then bilinearly upsampled and added.

\paragraph{Loss function} 
We use the non-saturating adversarial loss \cite{goodfellow2014generative} and regularize the discriminator with epsilon penalty \cite{karras2018progressive} and r1-regularization \cite{mescheder2018training}.
We mask the r1-regularization by $M$, similar to \cite{ConextualAttention2018Yu,hukkelaas2020image}, and apply it every 16th gradient step (known as "lazy regularization" \cite{karras2019analyzing}).
The total loss is given by
\begin{equation}
    \begin{aligned}
    \mathcal{L} = \mathcal{L}_{GAN} + \lambda_{EP} \cdot \mathcal{L}_{EP} + \lambda_{GP} \cdot \mathcal{L}_{GP} + 
        \lambda_{CSE} \mathcal{L}_{\text{CSE}}
    \end{aligned}
\end{equation}
where $\lambda_{EP}=0.001$, $\lambda_{GP}=5$, and $\lambda_{CSE} = 0.1$.
$\lambda_{EP}$ is identical to Progressive Growing GAN \cite{karras2018progressive}.
$\lambda_{GP}$ and $\lambda_{CSE}$ are determined by a rough hyperparameter search, where we tested $\lambda_{CSE} \in [.1, .2, .5, 1, 2, 5, 10, 50]$ and $\lambda_{GP} \in [0.1, 0.5, 5, 10, 20 ,100]$.
We did the hyperparameter search only on Config B.
No other hyperparameter search is done, unless stated otherwise.

\paragraph{Data Augmentation}
We use a limited amount of data augmentation, but find that it significantly improves quality of generated samples.
We adapt the augmentation pipeline of StyleGAN2-ada  \cite{karras2020ada} and modify the Pytorch implementation to support conditional image synthesis.
The pipeline includes general geometrical transformations, color transformations, rotation, and horizontal flip.
We significantly limit the amount of augmentation done, \eg we rotate by a maximum of $9^\circ$ left/right and translate by a maximum of 5\% of the image width/height.
This is to prevent augmentations leaking to our generator as we do not use adaptive augmentation training \cite{karras2020ada}.
Following the \href{https://github.com/NVlabs/stylegan2-ada-pytorch/blob/6f160b3d22b8b178ebe533a50d4d5e63aedba21d/training/augment.py#L117}{Pytorch implementation}, we use the following parameters;
rotate=0.5, rotate\_max=.05,
xint=.5, xint\_max=0.05,
scale=.5, scale\_std=.05,
aniso=0.5, aniso\_std=.05, 
xfrac=.5, xfrac\_std=.05,
brightness=.5, brightness\_std=.05,
contrast=.5, contrast\_std=.1,
hue=.5, hue\_max=.05,
saturation=.5, saturation\_std=.5,
imgfilter=.5, imgfilter\_std=.1.

\subsection{Face Quantitative Evaluation}
The quantitative evaluation of the face region was done by cropping the face region, upsampling the region to $(299, 299)$ and compute FID for every training sample in the dataset.
The face region was detected with DSFD \cite{li2018dsfd} using an open source Pytorch implementation \cite{hukkelasDSFD} where the highest scoring and largest face region was extracted.

\subsection{DeepFashion CSE-Dataset}
The DeepFashion CSE-dataset is derived from the In-shop Clothes Retrieval Benchmark of DeepFashion \cite{liu16DeepFashion}, where we have annotated each image with a CSE embedding.
Each image is automatically annotated with a pre-trained model from detectron2 \cite{wu2019detectron2}, specifically \href{https://github.com/facebookresearch/detectron2/blob/main/projects/DensePose/configs/cse/densepose_rcnn_R_101_FPN_DL_s1x.yaml}{R-101-FPN-DL-s1x}.
For each image, we select the highest scoring detected instance.
We remove any image that has no detections with a confidence score larger than 0.8.
The filtered dataset results in 40,625 training images and 10,275 validation images, where each image is downsampled to $384 \times 256$ using bilinear sampling.
We will include the train/val split that we randomly selected.

\paragraph{DeepFashion Decoder-Only Architecture}
The decoder-only generator is similar to the generator of StyleGAN2 \cite{karras2019analyzing}.
The generator consists of 6 residual blocks with two $3 \times 3$ convolutions each, where each block is followed by bilinear upsampling.
In total, the generator has $43.5$ M parameters, where each residual block has the following number of output channels: $[768, 768, 384, 192, 96, 48]$.
The starting resolution is $12 \times 8$ and the output is $384 \times 256$.

We use the same discriminator as for COCO-Body, except that we scale the number of parameters to 42.4M.
Otherwise, we use identical hyperparameters as for the COCO-Body dataset.
