# Supplementary material for: Realistic Full-Body Anonymization with Surface-Guided GANs
Source: arXiv:2201.02193 source file (2023-06-01)
Supplement: Supplementary file 3 [file full_metric_table.tex]

\begin{table*}[t]
    \caption{
        All quantitative metrics for every model in the main paper, where the leftmost column specify which table each model corresponds to.
        Note that some models are repeated in the table between different comparisons.
        Number of layers in the mapping network ($n$)  is 6 if not stated otherwise.
        }
    \label{tab:full_metric_table}
    \centering
    \begin{adjustbox}{width=\linewidth}
    \begin{tabular}{|l|l|c|c|c|c||c||c|c|c|}
        \hline
        && \multicolumn{4}{c||}{Main Metrics} & \multicolumn{1}{c||}{Face Metric} & \multicolumn{3}{c|}{PSNR Affine Transformation} \\
        &Model & LPIPS $\downarrow$ &  LPIPS Diversity $\uparrow$ & FID $\downarrow$ & PPL $\downarrow$  & FID $\downarrow$ & Translation $\uparrow$ & Hflip $\uparrow$ & Rotation $\uparrow$ \\
        \hline
        \hline
        \multirow{5}{*}{\rotatebox[origin=c]{90}{Table 1}} &A (Baseline) & 0.237 & 0.162 & 7.4   & 26.7  & 13.4  & 22.0  & 20.4  & 19.3  \\
        \cline{2-10}
        &B (A+ CSE Supervision)         & 0.220 & 0.140 & 5.8   & 19.0  & 9.1   & 23.1  & 21.7  & 20.3  \\
        \cline{2-10}
        &C, \modulationMetodShort     & 0.219 & 0.143 & 5.6   & 19.2  & 7.4   & 23.8  & 21.4  & 20.7  \\
        \cline{2-10}
        &D, \modulationMetodNoiseShort & 0.220 & 0.166 & 5.2   & 13.7  & 7.4   & 26.1  & 22.5  & 21.4  \\
        \cline{2-10}
        & E, Larger D/G                              & 0.211 & 0.161 & 4.8   & 15.1  & 6.8   & 26.2  & 22.1  &  21.0 \\
        \hline
        \hline
        \multirow{5}{*}{\rotatebox[origin=c]{90}{Table 2}} & D, \modulationMetodNoiseShort $n$=0 & 0.221 & 0.155 & 5.4   & 24.9  & 7.7   & 25.9  & 22.0  & 21.1  \\
        \cline{2-10}
        &D, \modulationMetodNoiseShort $n$=2  & 0.221 & 0.164 & 5.4   & 19.7  & 8.0   & 26.1  & 21.9  & 21.3  \\
        \cline{2-10}
        &D, \modulationMetodNoiseShort $n$=4 & 0.221 & 0.161 & 5.5   & 19.8  & 7.9   & 26.0  & 22.0  & 21.1  \\
        \cline{2-10}
        &D, \modulationMetodNoiseShort $n$=6 & 0.220 & 0.166 & 5.2   & 13.7  & 7.4   & 26.1  & 22.5  & 21.4  \\
        \hline
        \hline
        \multirow{5}{*}{\rotatebox[origin=c]{90}{Table 3}} &B + SPADE \cite{Park_2019}   &   0.223 & 0.150 & 5.9   & 20.6  & 9.7   & 22.5  & 20.7  & 19.8  \\
        \cline{2-10}
        &B + CLADE \cite{Tan_2021CLADE} & 0.221 & 0.138 & 5.7   & 16.9  & 8.9   & 22.9  & 21.3  & 20.1  \\
        \cline{2-10}
        &B + INADE \cite{tan2021INADE} & 0.223 & 0.140 & 5.8   & 19.5  & 9.4   & 24.1  & 20.9  & 20.2  \\
        \cline{2-10}
        & B + StyleGAN \cite{karras2019analyzing} &  0.220 & 0.155 & 5.7   & 48.2  & 9.4   & 25.5  & 21.6  & 20.9  \\
        \cline{2-10}
        & B + CoMod  & 0.221 & 0.154 & 5.5  & 17.9 &  17.5   &   24.5  &  21.6   &   20.6  \\
        \hline
    \end{tabular}
    \end{adjustbox}
\end{table*}
