# Supplementary material for: Realistic Full-Body Anonymization with Surface-Guided GANs
Source: arXiv:2201.02193 source file (2023-06-01)
Supplement: Supplementary file 4 [file quantitative.tex]

\begin{figure*}[t]
    \centering
    \begin{subfigure}[t]{.5\linewidth}
        \includegraphics[width=\linewidth]{figures/truncation.pdf}
        \caption{}
    \end{subfigure}%%
    \begin{subfigure}[t]{.5\linewidth}
        \includegraphics[width=\linewidth]{figures/truncation_w_interpolation.pdf}
        \caption{}
    \end{subfigure}%%
    \caption{
        Analysis of truncation techniques for \modulationMetodNoiseShort .
        \textbf{(a)} Compares different truncation strategies applied to the intermediate latent space $\omega$ or $z$. Truncation in $\omega$ yields a better trade off between diversity and image quality.
        \textbf{(b)} Evaluates the effect of $\omega$ interpolation , where we interpolate a sampled latent towards $\bar{\omega}$. Increasing the truncation (t) gradually improves image quality at the cost of sample diversity.
        }
    \label{fig:truncation_experiment}
\end{figure*}
\section{Additional Quantitative Results}
\Cref{tab:full_metric_table} includes all metrics for every model that is reported in the main paper.
\label{sec:appendix_quantitative}
\subsection{Truncation Trick}

The truncation trick is an established technique to sample latent vectors from a truncated distribution to improve generated image quality at the cost of diversity of samples \cite{Brock2018}.
A similar strategy is adopted for the intermediate latent space of StyleGAN \cite{karras2019style}, which is shown to be more effective than truncating in $z$  \cite{kynkaanniemi2019improvedPrecision}.

We adopt a similar strategy \cite{karras2019style,kynkaanniemi2019improvedPrecision} for the conditional latent space of \modulationMetodNoiseShort .
We find the mass of center; $\bar{\omega_i} = \mathbb{E}_{z \sim P(z)} [f_\omega (\omega_i,z)]$.
Then, we evaluate the effect of interpolation and \text{clamp}ing the latent by the following apporaches;
\begin{itemize}
    \item \textbf{Interpolate $\omega$}: $\bar{\omega} + t_i \cdot (\omega - \bar{\omega})$,
    \item \textbf{Clamp $\omega$}: $\text{clamp}(\omega, \bar{\omega} - t_c, \bar{\omega} + t_c)$,
    \item \textbf{Interpolate $z$}: $ t_i \cdot z$,
    \item \textbf{Clamp $z$}: $\text{clamp}(z, -t_c, t_c)$\,
\end{itemize}
where $t_i \in \mathbb{R}, t_i \in [0, 1]$, and  $\text{clamp}(x,x_{\text{lower}}, x_{\text{upper}})$ sets all elements of $x$ that are outside the range of $[x_{\text{lower}}, x_{\text{upper}}]$ to $x_{\text{lower}}$ or  $x_{\text{upper}}$.

We observe that truncating the intermediate latent space $\omega$ yields a better tradeoff between quality and diversity, compared to truncating in $z$ (\Cref{fig:truncation_experiment}).

\paragraph{Interpolating in $\omega$}
The disentangled representation of \modulationMetodNoiseShort allows for natural transitions between different synthesized styles.
\Cref{fig:interpolation_example} reflects that linearly interpolating between two randomly sampled $\omega$ yields a natural transition.
Observe that the interpolation path is smooth, where different features of the synthesized person is gradually changed.
Note that we observe a discontinuous transition (\eg Row 5 in \Cref{fig:interpolation_example}) for some combinations of conditional pose and sampled $\omega$.
We speculate that  a deeper mapping network can further improve the disentanglement and mitigate this non-smooth transition.

\begin{figure}[t]
    \centering
    \includegraphics[width=\linewidth]{figures/interpolation_example.png}
    \caption{
        Example of latent interpolation in the intermediate latent space $\omega$.
        The images are generated with linear interpolation between two randomly sampled $\omega$, starting from 0 (leftmost column) to 1 (rightmost column).
        Each row is generated with different latents.
        No latent truncation is done.}
    \label{fig:interpolation_example}
\end{figure}

\subsection{Effect of Anonymization for Computer Vision}
\begin{table}
    \caption{
        Object Detection AP on the PASCAL VOC validation set \cite{everingham10pascal}.
        The results are from a \textbf{pre-trained} Faster R-CNN \cite{ren2015faster} \href{https://github.com/facebookresearch/detectron2/blob/335b19830e4ea5c5a74a085a04ff4a2f1a1dbf71/configs/PascalVOC-Detection/faster_rcnn_R_50_C4.yaml}{R50-C4} from detectron2 \cite{wu2019detectron2}.
        }
    \label{tab:pascal_val}
    \centering
    \begin{adjustbox}{max width=\linewidth}
    \begin{tabular}{|c|c|c|c|}
        \hline
        \textbf{Validation} Dataset & AP$_{50:95}$ $\uparrow$ & AP$_{50}$ $\uparrow$ & AP$_{75}$ $\uparrow$ \\
        \hline
        \hline
        Original                       & 51.8                           & 80.3                           & 56.5   \\
        \hline
        \hline
        Mask Out        & 47.9                           & 75.2                           & 51.4   \\ 
        \hline
        $8 \times 8$ Pixelation        & 47.2                           & 75.1                           & 50.8   \\
        \hline
        $16 \times 16$ Pixelation        & 48.5                           & 76.7                           & 52.0   \\
        \hline
        Ours        & \textbf{50.3}                           & \textbf{78.9}                           & \textbf{54.2}   \\
        \hline
    \end{tabular}
    \end{adjustbox}
\end{table}
\begin{table*}[t]
    \caption{
        Instance segmentation mask AP on the COCO validation set \cite{lin2014microsoft}.
        The results are from a Mask R-CNN \cite{he2017mask} \href{https://github.com/facebookresearch/detectron2/blob/335b19830e4ea5c5a74a085a04ff4a2f1a1dbf71/configs/COCO-InstanceSegmentation/mask_rcnn_R_50_FPN_3x.yaml}{R50-FPN-3x} from detectron2 \cite{wu2019detectron2} trained on different anonymized datasets.
        The validation set is not anonymized.
        }
    \label{tab:coco_training}
    \centering
    \begin{tabular}{|c|c|c|c|c|c|c|c|}
        \hline
        \textbf{Training} Dataset & AP$_{50:95}$ $\uparrow$ & AP$_{50}$ $\uparrow$ & AP$_{75}$ $\uparrow$ & AP$_{\text{s}}$ $\uparrow$ & AP$_{\text{m}}$ $\uparrow$& AP$_{\text{l}}$ $\uparrow$ & AP$_\text{Person}$ $\uparrow$ \\
        \hline
        \hline
        Original                       & 37.1                           & 58.7                           & 39.8                           & 18.8                           & 39.6                           & 53.3                           & 47.8                           \\
        \hline
        \hline
        Mask Out                       & 34.6                           & 55.2                           & 36.7                           & 16.7                           & 36.5                           & 50.0                           & 44.7                           \\
        \hline
        $8 \times 8$ Pixelation        & 34.8                           & 55.7                           & 37.0                           & 16.9                           & \textbf{36.7}                           & 50.3                           & 46.5                           \\
        \hline
        $16 \times 16$ Pixelation      & \textbf{35.0}                           & 55.9                           & 37.3                           & 17.3                           & 37.1                           & 50.4                           & \textbf{46.9}                           \\
        \hline
        Ours                           & \textbf{35.0}                           & \textbf{56.0}                           & \textbf{37.5}                           & \textbf{17.7}                           & \textbf{36.7}                           & \textbf{50.6}                           & 46.5                           \\
        \hline
    \end{tabular}
\end{table*}
\begin{table}
    \caption{
        Object Detection AP on the PASCAL VOC validation set \cite{everingham10pascal}.
        The results are from a Faster R-CNN \cite{ren2015faster} \href{https://github.com/facebookresearch/detectron2/blob/335b19830e4ea5c5a74a085a04ff4a2f1a1dbf71/configs/PascalVOC-Detection/faster_rcnn_R_50_C4.yaml}{R50-C4} from detectron2 \cite{wu2019detectron2} trained on different anonymized datasets.
        The validation set is not anonymized.
        }
    \label{tab:pascal_train}
    \centering
    \begin{tabular}{|c|c|c|c|}
        \hline
        \textbf{Training} Dataset & AP$_{50:95}$ $\uparrow$ & AP$_{50}$ $\uparrow$ & AP$_{75}$ $\uparrow$ \\
        \hline
        \hline
        Original                       & 51.8                           & 80.3                           & 56.5   \\
        \hline
        \hline
        Mask Out        & \textbf{51.3}                           & 80.0                           & 55.7   \\
        \hline
        $8 \times 8$ Pixelation        & 51.2                           & 79.9                           & 55.03   \\
        \hline
        $16 \times 16$ Pixelation        & 51.2                           & 79.8                           & 55.7   \\
        \hline
        Ours        & \textbf{51.3}                           & \textbf{80.1}                           & \textbf{56.0}   \\
        \hline
    \end{tabular}
\end{table}

\paragraph{Anonymizing Data for Evaluation (PASCAL VOC)}
Following the same approach as for COCO (described in the main paper), we show that surface-guided anonymization strongly improves over traditional techniques for evaluation purposes (\Cref{tab:pascal_val}).
Furthermore, we note a slight gap between surface-guided anonymization and the original dataset (50.3 vs 51.8 AP).
We believe this originates primarily from errors in detection, as we use a confidence threshold of 0.1.

\paragraph{Anonymizing data for Training}
Surface-guided anonymization slightly improves over traditional anonymization when using the anonymized data for training (\Cref{tab:coco_training}, \Cref{tab:pascal_train}).
Our naive anonymization of COCO without modifying object labels (\eg not removing the class "tie") introduces ambiguities in the training objective, which we believe significantly degrades training performance.
This issue is not as severe for pixelation, as these objects are still present in the image.
Furthermore, we note that the CSE detector has several false positives and negatives which directly impacts the training objective.
For example, false positives yields highly corrupted images with surface-guided anonymization.
