# Supplementary material for: Realistic Full-Body Anonymization with Surface-Guided GANs
Source: arXiv:2201.02193 source file (2023-06-01)
Supplement: Supplementary file 5 [file qualitative.tex]

\section{Additional Qualitative Results}
\label{sec:appendix_qualitative}

\subsection{COCO-Body}
Random examples from the COCO-Body dataset are given in \Cref{fig:random_cse1}, \Cref{fig:random_cse2}, \Cref{fig:random_cse3}, and \Cref{fig:random_cse4}.

\subsection{DeepFashion}
Random examples from the DeepFashion-CSE dataset are given in \Cref{fig:random_DF1}, \Cref{fig:random_DF2}, and \Cref{fig:random_DF3}.

\subsection{COCO}
Random examples from the COCO dataset are given in \Cref{fig:coco_random1}, \Cref{fig:coco_random2}, \Cref{fig:coco_random3}, \Cref{fig:coco_random4}, \Cref{fig:coco_random5} and \Cref{fig:coco_random6}.
